# Supplementary material for: Fast Converging Anytime Model Counting
Source: arXiv:2212.09390 source file (2022-12-19)
Supplement: Supplementary file 1 [file Appendix.tex]

\newpage
\appendix
\section{Appendix}\label{stylefiles}
\subsection{Proofs}
\label{app:proofs}

We now present proofs of Propositions \ref{prop:exact-bound} and \ref{prop:PartialKC}.

\PropBound*
\begin{proof}
	Due to the duality, we only show the case for the lower bound.
	It is easy to see the case for the leaf nodes. 	
	For a full CCDD, its model count can be computed as follows \cite{Lai:etal:21}:
	\begin{equation}\label{eq:exact-count}
	Z(u) = \begin{cases}
		0 & sym(u) = \bot \\
		2^{|X|} & sym(u) = \top \\
		c^{-1} \cdot \prod_{v \in Ch(u)}Z(v) & sym(u) = \land_d  \\
		\dfrac{Z(ch_{\mathit{core}}(u))}{2^{|Ch(u)| - 1}} & sym(u) = \land_k  \\
		\dfrac{Z(ch_0(u)) + Z(ch_1(u))}{2} & {\text{otherwise}}
		\end{cases}
	\end{equation}
	Therefore, we can immediately prove this proposition by induction.
	We assume that this proposition holds with the number of nodes $|V(\D_u)| \le m$. When $|V(\D_u)| = m + 1$, we proceed by case analysis:
	\begin{itemize}
		\item For a decision node $u$, we have $\widetilde{Z}(ch_0(u) \le Z(ch_0(u))$ and $\widetilde{Z}(ch_1(u) \le Z(ch_1(u))$.
		Thus, $\widetilde{Z}(u) = \dfrac{\widetilde{Z}(ch_0(u)) + \widetilde{Z}(ch_1(u))}{2} \le \dfrac{Z(ch_0(u)) + Z(ch_1(u))}{2} = Z(u)$.
		\item For a decomposed node $u$, we have $\widetilde{Z}(v) \le Z(v)$ for each child. Thus, $\widetilde{Z}(u) = c^{-1} \cdot \prod_{v \in Ch(u)}\widetilde{Z}(v) \le c^{-1} \cdot \prod_{v \in Ch(u)}Z(v) = Z(u)$.
		\item For a kernelized node $u$, we have $\widetilde{Z}(ch_{core}(u)) \le Z(ch_{core}(u))$. Thus, $\widetilde{Z}(u) =  \dfrac{\widetilde{Z}(ch_{\mathit{core}}(u))}{2^{|Ch(u)| - 1}} \le \dfrac{Z(ch_{\mathit{core}}(u))}{2^{|Ch(u)| - 1}} = Z(u)$
	\end{itemize}
	
\end{proof}
\PropPartialKC*

\begin{proof}
%	It is easy to see that 
If \PartialKC{} exceeds memory limits, it just restarts. Finally, \PartialKC{} returns the average estimate. Therefore, we just show when \PartialKC{} does not exceed memory, it outputs an unbiased estimate of the model count for a given formula.
	
	Given the input $\varphi$, we denote all of the inputs of recursively calls of \MicroKC{} as a sequence $S = (\varphi_1, \ldots, \varphi_n=\varphi)$ in the call of \PartialKC($\varphi$, $t$).
	Let $N$ be the final number of calls of \MicroKC{} on $\varphi$.
	
	We first prove the case $N=1$.
	We prove by induction with the hypothesis that the call of \MicroKC($\psi$) returns an unbiased estimate of the model count of $\psi$ if $|\Vars(\psi)| < |\Vars(\varphi_n)|$. Thus, the calls of \MicroKC{} on $\varphi_1, \ldots, \varphi_{i-1}$ return an unbiased estimate of the model counts, and the results are stored in $Cache$.
	We denote the output of \MicroKC($\varphi_i$) by $u_i$.
	The case when \MicroKC{} returns a leaf node is obvious.
	It is obvious that $\Cache(\varphi_n) = nil$ in line 4.
	We proceed by a case analysis:
	\begin{enumerate}[(a)]
		\item $E \not= \emptyset$ in line 6: The input of the recursive call is $\varphi_{n-1}$. According to the induction hypothesis, $\Expectation{}{\widehat{Z}(v)} = Z(\varphi_{n-1})$. Thus, $\Expectation{}{\widehat{Z}(u_n)} =  \dfrac{Z(\varphi_{n-1})}{2^{|Ch(u)| - 1}} = Z(\varphi_{n})$ (see Proposition 1 in \cite{Lai:etal:21}).
		\item $|\Psi| = m > 1$ on line 15: The input of the recursive calls are $\varphi_{n-m}, \ldots, \varphi_{n-1}$. According to the induction hypothesis, $\Expectation{}{\widehat{Z}(u_i)} = Z(\varphi_{i})$ ($n-m \le i \le n-1$). Due to the conditional independence, $\Expectation{}{\widehat{Z}(u_n)} =  c^{-1} \cdot \prod_{n-m \le i \le n-1}\Expectation{}{\widehat{Z}(u_i)} = c^{-1} \cdot \prod_{n-m \le i \le n-1}Z(\varphi_i) = Z(\varphi_{n})$.
		\item $|\Psi| = 1$ on line 15. The input of the recursive call is $\varphi_{n-2} = \varphi_n[x \mapsto false]$ and $\varphi_{n-1} = \varphi_n[x \mapsto true]$. Thus, $Z(\varphi_{n}) = \frac{1}{2} \cdot (Z(\varphi_{n-2}) + Z(\varphi_{n-1}))$. 
		\begin{align*}
			\Expectation{}{\widehat{Z}(u)}&=\frac{\Expectation{}{\widehat{Z}(ch_0(u))} \cdot f_0(u)}{2p_0(u) \cdot (f_0(u) + f_1(u))} \cdot p_0(u)+\\
			&\mathrel{\phantom{=}}\frac{\Expectation{}{\widehat{Z}(ch_1(u))}\cdot f_1(u)}{2p_1(u) \cdot (f_0(u) + f_1(u))} \cdot p_1(u)\\
			&=\frac{1}{2} \cdot \left(\Expectation{}{\widehat{Z}(ch_0(u))} + \Expectation{}{\widehat{Z}(ch_1(u))}\right)\\
			&=Z(\varphi_{n}).
		\end{align*}
	\end{enumerate}

	We can also prove the case $N > 1$ by induction.
	It is easy to see that we call \MicroKC{} on the same formula at most $N$ times; in other words, each formula in $S$ at most $N$ times.
	It is assumed that the $M$-th call of \MicroKC($\psi$) returns an unbiased estimate of the model count of $\psi$ if $|\Vars(\psi)| < |\Vars(\varphi_n)|$ or $M < N$. 
	Then the proof for this case is similar to the case $N=1$ except the decision case. 
	We remark that for a decision node without any unknown node, we can compute its exact count by applying Eq. \eqref{eq:bound}.
	When it returns a known node in lines 42--43, we can get the exact count.
	Now we prove the case when non-unknown node is returned.
	For convenience, we denote the returned node by $u$.
	The value of $f(u)$ is independent from what are the children of $u$. 
	We have $\Expectation{}{\frac{f_0(u)}{N}}=p_0(u)$ and $\Expectation{}{\frac{f_1(u)}{N}}=p_1(u)$. According to the decision case of Eq. \eqref{eq:unbiased}, we have the following equation:
	\begin{align*}
		\Expectation{}{\widehat{Z}(u)}&=\frac{\Expectation{}{\widehat{Z}(ch_0(u))} \cdot \Expectation{}{f_0(u)}}{2p_0(u) \cdot N} +\\
		&\mathrel{\phantom{=}}\frac{\Expectation{}{\widehat{Z}(ch_1(u))}\cdot \Expectation{}{f_1(v)}}{2p_1(u) \cdot N}+\\
		&=\frac{1}{2} \cdot \left(\Expectation{}{\widehat{Z}(ch_0(u))} + \Expectation{}{\widehat{Z}(ch_1(u))}\right)\\
		&=Z(\varphi_{n}).
	\end{align*}
\end{proof}

\subsection{Algorithm \MargProb}
\label{app:MargProb}

The Algorithm \MargProb{} is presented in Algorithm \ref{alg:MargProb}. In \MargProb{}, we first perform two projected knowledge compilations by \ProjectedKC{} in Algorithm \ref{alg:ProjectedKC}, and then use the compiled results to compute the marginal probability by using Eq. \eqref{eq:exact-count}.
\ProjectedKC{} returns a CCDD. Since the projected set $P$ we use is small, and the kernelization itself has a time cost, we do not use kernelization.

\begin{algorithm}[tb]
	\caption{\MargProb($\varphi$, $x$)} \label{alg:MargProb}
	$u \leftarrow \ProjectedKC(\varphi[x \mapsto false], P)$\;
	$v \leftarrow \ProjectedKC(\varphi[x \mapsto true], P)$\;
	\KwRet $\frac{Z(v)}{Z(u)+Z(v)}$
\end{algorithm}

\begin{algorithm}[tb]
	\caption{\ProjectedKC($\varphi$, $P$)} \label{alg:ProjectedKC}
	\lIf {$\varphi = \mathit{false}$} {\KwRet $\Angle{\bot}$} \label{line:ProjectedKC:base-case-begin}
	\lIf {$\varphi = \mathit{true}$} {\KwRet $\Angle{\top}$} \label{line:ProjectedKC:base-case-end}
	\lIf {$\mathit{ProjCache}(\varphi) \not= nil$} {\KwRet $\mathit{ProjCache}(\varphi)$}
	$\Psi \leftarrow \Decompose(\varphi)$\; \label{line:ProjectedKC:decompose}
	\uIf {$|\Psi| > 1$} {
		$W \leftarrow \{\ProjectedKC(\psi ) \mid \psi \in \Psi\}$\;
		\KwRet $\mathit{ProjCache}(\varphi) \leftarrow \Angle{\land_d, W}$\label{line:ProjectedKC:decomposition}
	}
	\Else{ 
		\If{ $\Vars(\varphi) \cap P = \emptyset$  }{
			\lIf {$\varphi$ is satisfiable} {\KwRet $\Angle{\top}$}
			\lElse {\KwRet $\Angle{\bot}$} 
		}
		$x \leftarrow \PickGoodVar(\varphi, P)$\; \label{line:ProjectedKC:decision-begin}
		$w_0 \leftarrow \ProjectedKC(\varphi[x \mapsto false])$\;
		$w_1 \leftarrow \ProjectedKC(\varphi[x \mapsto true])$\; 
		\KwRet $\mathit{ProjCache}(\varphi) \leftarrow \Angle{x, w_0, w_1}$\; \label{line:ProjectedKC:decision-end}
	}
\end{algorithm}

\subsection{Discussion on the effect of decomposition for reducing variance}
\label{app:variance}

In detail, we can use decomposition to reduce the variance of \PartialKC{} from the following three aspects:

\begin{compactitem}[$\bullet$]
	\item After extracting all implied literals, on the one hand, we can reduce the number of sampling Boolean values from the Bernoulli distributions. On the other hand, for each $\psi$ in line 16 with more than one variable and each variable $x \in Vars(\psi)$, we have that $\psi \not\models \lnot x$ and $\psi \not\models x$. Thus, sampling in lines \ref{line:MicroKC:initial-sample} and \ref{line:MicroKC:repeat-sample} is backtrack-free, which remedies the rejection problem of sampling.
	\item Similar to the approach in \cite{Gogate:Dechter:11}, we reduce the variance by sampling from a subset of the variables, a technique also known as Rao-Blackwellization. In line 3 in Algorithm \textsc{PartialKC}, we call a exact counter to compute the exact count if a CNF formula is easy detected by \EasyInstance{}. After decomposing, we can detect more than one easy formula in each calling of \MicroKC{}, and therefore greatly reduce the variance.
	\item After decomposing, more virtual samples can be provided in contrast to the original samples \cite{Gogate:Dechter:12}. For example, sampling twice for each sub-formula in line 16 or 35
	yields $2^n$ virtual samples. Compared with the static decomposition scheme use in \cite{Gogate:Dechter:12}, the dynamic decomposition scheme used in our implementation may provide a finer decomposition for the same formula. Therefore, more virtual samples can be provided to reduce the variance with a finer decomposition.
\end{compactitem}
